# Supplementary material for: Optimal Semantic-aware Sampling and Transmission in Energy Harvesting Systems Through the AoII
Source: arXiv:2304.00875 source file (2023-11-11)
Supplement: Supplementary file 1 [file Appendix.tex]

\appendix

\subsection{Proof of Proposition  \ref{Prop_ComMDP}}\label{App_ComMDP}
First, we show the former via a counterexample. 
Specifically, we show the
the following deterministic policy induces a Markov chain with two recurrent classes, contradicting the unichain structure.
%Without loss of generality, suppose the battery capacity $E=5$.
The policy works as follows: it takes a new sample and transmits it whenever the energy level $e(t)$ is $3$; otherwise, it chooses the idle action. 
In the induced Markov chain, the set of states ${ \{ (e,\theta)\}_{\{e\le 3,\, \theta=1,2,\dots,N\}} },$ and 
${ \{ (E,N)\} },$
are two different recurrent classes, and 
the set of states ${ \{ (e,\theta)\}_{\{e > 3,\, \theta\neq N\}} },$ are transient states. Thus, the Markov chain has more than one recurrent class, which completes the first part of proof.
%The induced Markov chain for the $e(t)$ is shown in Fig. \ref{Fig_CEx}, which is multichain.

To show the MDP is communicating, by \cite[Proposition 8.3.1]{Puterman_Book}, it is sufficient to find a randomized policy which induces a recurrent Markov chain, i.e., 
a policy  under which every pair of states ${s=(e,\theta)}$ and ${ s'=(e',\theta')}$ in $\mathcal{S}$ is accessible from each other.
We define the following policy: the policy takes the idle action $a(t) =0$ (w.p.1.) at any state in which
${ e(t) < c }$,
%$(e(t) < c^{\mathrm{s}} + c^{\mathrm{t}}, \theta(t))$, 
and  takes the idle action w.p. $0.5$ in the other states. 
For the case where $e' \ge e$, realizing the idle action for at least ${ e' - e + c } $ consecutive slots, starting from $(e,\theta)$, leads to state ${(\min\{e' - e + c, E\}, \min\{\theta +e' - e + c, N \}) }$ w.p.p.;
then the action $a(t) = 1$ leads to state $(e', 1)$ w.p.p., and 
subsequently the idle action $a = 0$ for $\theta'-1$ consecutive
slots leads to state $(e',\theta')$ w.p.p.. 
Similarly, for the case where $e' < e$, supposing $e\ge c$ without loss of generality,  taking action $a = 1$ for at least ${ \floor{\frac{e }{c  } } } $ consecutive slots leads 
  to state $(r\triangleq e-c\floor{\frac{e }{c }}, 1)$ w.p.p.; then taking the idle action $a = 0$ for at least  $c-r$ slots leads to state $(0, \min\{1+c-r, N\})$. Now, following the same procedure for the first case $e'\ge e$, where $e=0$,  leads to state $(e',\theta') $ w.p.p., which completes the proof. 
